# Supplementary material for: A "lighthouse" laser-driven staged proton accelerator allowing for ultrafast angular and spectral control
Source: arXiv:2404.11321 source file (2024-04-17)
Supplement: Supplementary file 1 [file suppPRL.tex]

\documentclass[%
%preprint,
%article,
superscriptaddress,
%groupedaddress,
%unsortedaddress,
%runinaddress,
%frontmatterverbose, 
%twocolumn,
%preprint,
%showpacs,preprintnumbers,
nofootinbib,
%linenumbers,
notitlepage,
%nobibnotes,
%bibnotes,
amsmath,amssymb,
% aps,
%aip,
%showkeys,
%pop,
%prl,
%jmp,
%prstab,
%prstper,
%floatfix,
]{revtex4-1}

% Page geometry
\usepackage[a4paper,margin=2.5cm]{geometry}
\usepackage{graphicx}% Include figure files
\usepackage{upgreek}

\newcommand{\degr}{$^\circ$}
\usepackage[table,xcdraw]{xcolor}
\setcounter{figure}{0}

% Your additional packages and settings can go here

\begin{document}

\title{Supplementary Material: A ``lighthouse'' laser-driven staged proton accelerator allowing for ultrafast angular and spectral control}

\author{V. Horný}
\email{vojtech.horny@eli-np.ro}
\affiliation{LULI - CNRS, CEA, Sorbonne Université, Ecole Polytechnique, Institut Polytechnique de Paris - F-91128 Palaiseau cedex, France}
\affiliation{CEA, DAM, DIF, 91297 Arpajon, France}
\affiliation{Université Paris-Saclay, CEA, LMCE, 91680 Bruyères-le-Châtel, France}
\affiliation{ELI NP, ”Horia Hulubei” National Institute for Physics and Nuclear Engineering, 30 Reactorului Street, RO-077125, Bucharest-Magurele, Romania}
\author{K. Burdonov}
\affiliation{LULI - CNRS, CEA, Sorbonne Université, Ecole Polytechnique, Institut Polytechnique de Paris - F-91128 Palaiseau cedex, France}
\affiliation{Sorbonne Université, Observatoire de Paris, Université PSL, CNRS, LERMA, F-75005, Paris, France}
\author{A. Fazzini}
\affiliation{LULI - CNRS, CEA, Sorbonne Université, Ecole Polytechnique, Institut Polytechnique de Paris - F-91128 Palaiseau cedex, France}
\author{V. Lelasseux}
\affiliation{LULI - CNRS, CEA, Sorbonne Université, Ecole Polytechnique, Institut Polytechnique de Paris - F-91128 Palaiseau cedex, France}
\affiliation{ELI NP, ”Horia Hulubei” National Institute for Physics and Nuclear Engineering, 30 Reactorului Street, RO-077125, Bucharest-Magurele, Romania}
\author{P. Antici}
\affiliation{INRS-EMT, 1650, boulevard Lionel-Boulet, J3X 1S2, Varennes (Québec), Canada}
\author{S.N. Chen}
\affiliation{ELI NP, ”Horia Hulubei” National Institute for Physics and Nuclear Engineering, 30 Reactorului Street, RO-077125, Bucharest-Magurele, Romania}
\author{A. Ciardi}
\affiliation{Sorbonne Université, Observatoire de Paris, Université PSL, CNRS, LERMA, F-75005, Paris, France}
\author{X.~Davoine}
\affiliation{CEA, DAM, DIF, 91297 Arpajon, France}
\affiliation{Université Paris-Saclay, CEA, LMCE, 91680 Bruyères-le-Châtel, France}
\author{E.~d'Humières}
\affiliation{Université de Bordeaux, CNRS, CEA, CELIA (Centre Lasers Intenses et Applications), UMR 5107, Talence, France}
\author{L. Gremillet}
\affiliation{CEA, DAM, DIF, 91297 Arpajon, France}
\affiliation{Université Paris-Saclay, CEA, LMCE, 91680 Bruyères-le-Châtel, France}
\author{L.~Lecherbourg}
\affiliation{CEA, DAM, DIF, 91297 Arpajon, France}
\affiliation{Université Paris-Saclay, CEA, LMCE, 91680 Bruyères-le-Châtel, France}
\author{F. Mathieu}
\affiliation{LULI - CNRS, CEA, Sorbonne Université, Ecole Polytechnique, Institut Polytechnique de Paris - F-91128 Palaiseau cedex, France}
\author{D. Papadopoulos}
\affiliation{LULI - CNRS, CEA, Sorbonne Université, Ecole Polytechnique, Institut Polytechnique de Paris - F-91128 Palaiseau cedex, France}
\author{W. Yao}
\affiliation{LULI - CNRS, CEA, Sorbonne Université, Ecole Polytechnique, Institut Polytechnique de Paris - F-91128 Palaiseau cedex, France}
\affiliation{Sorbonne Université, Observatoire de Paris, Université PSL, CNRS, LERMA, F-75005, Paris, France}
\author{J. Fuchs}
\email{julien.fuchs@polytechnique.edu}
\affiliation{LULI - CNRS, CEA, Sorbonne Université, Ecole Polytechnique, Institut Polytechnique de Paris - F-91128 Palaiseau cedex, France}

\date{\today}

\maketitle

\section{Hydrodynamical simulation}

Figure~\ref{figC} illustrates the longitudinal density profiles (normalized to the critical density $n_c$) of the expanding electron (blue solid line) and ion (orange solid line) components of the foil target, as extracted at the end of the hydrodynamical simulation ($t=-1\,\rm ps$ relative to the laser peak). At this point, the critical-density surface ($n_e=n_c$) has shifted approximately 2--$3,\rm \upmu m$ away from the initial target surface (black dashed line), with a local density scale-length $(\partial \ln n_e /\partial x)^{-1} \simeq 2\,\rm \upmu m$. The shock initiated within the target bulk appears as a density peak located at $x\simeq 0.4\,\rm \upmu m$.

\begin{figure}[h]
    \centering
    \includegraphics{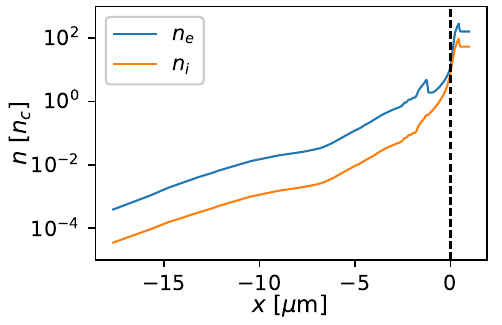}
    \caption{
    Longitudinal electron (blue) and ion (orange) density profiles 1~ps before the pulse maximum, as predicted by a 1D \textsc{esther} hydrodynamic simulation using the measured temporal laser profile \cite{burdonov2021characterization}. The dashed line locates the unperturbed target front surface.
    }
    \label{figC}
\end{figure}

\section{Numerical parameters of the PIC simulation}
The plasma evolution within the last picosecond before the pulse maximum and the associated ion acceleration are simulated by the particle-in-cell (PIC) method, employing the 2D3V (2D in space, 3D in momentum space) version of the \textsc{calder} code \cite{lefebvre2003electron}. The numerical domain, of dimensions $L_x \times L_y = 50.93 \times 61.11\,\rm \upmu m^2$, is discretized into $10\,000 \times 12\,000$ cells of size $\Delta x = \Delta y = 5.093\,\rm nm$. The laser pulse is injected from the left-hand side and focused at 45\degr incidence to a $3\,\rm \upmu m$ full-width-at-half-maximum spot located at $(x_f, y_f)=(20,0)\,\rm \upmu m$, corresponding to the unperturbed target surface. The temporal laser intensity profile reproduces that plotted in Fig.~1(b) in the main text.

The density profile of the plasma Al ions ($n_i$) in the longitudinal direction is taken from the hydrodynamic simulation, while it is assumed uniform in the transverse direction. To mitigate spurious numerical heating throughout the ps simulation timescale, the electron and ion temperatures are set to 0.1~eV everywhere while the ion charge state is set to $Z^\star = 3$. Accordingly, the electron density profile is initialized to $n_e = Z^\star n_i$. This simplification is justified because the intense rising edge of the laser profile will rapidly bring the plasma to a higher ionization state consistent with the experimental reality. In addition, a $2\Delta x$ thick layer of hydrogen atoms of density $n_p=60\,n_c$ is attached to the target backside, modeling the surface contaminants from which protons are accelerated. The Al, H and electron species are initially represented by 4, 1000 and 4 macroparticles per cell, respectively. Elastic collisions between all plasma species and electron impact ionization \cite{perez2012} are described along with field-induced ionization \cite{nuter2011}. To further reduce numerical heating, fourth-order weight factors and the Godfrey-Vay \cite{godfrey2014} and Friedman \cite{greenwood2004elimination} filtering schemes are used. Moreover, a two-pass compensated binomial filter is applied to smooth the current density.

\section{Discussion of the 2D simulation geometry accuracy}
Our simulations replicate the physics behind the observed proton beam bending, yet the energy of the fastest protons from 1--$5\,\rm \upmu m$ thick targets lies in the $\sim 50$--$60\,\rm MeV$ range [see Fig.~4(b) in the main text], about twice that observed in the experiment. This difference can be attributed to the idealized (Gaussian) transverse envelope of the laser beam and, above all, to the simplified (2D) simulation geometry, which is known to overestimate the efficiency of TNSA \cite{sgattoni2012laser, takagi2021multivariate}. This discrepancy likely accounts for the underestimated proton deviation seen in the simulation, as the longitudinal acceleration field is overestimated. Unfortunately, a full 3D simulation with the required resolution and duration is still beyond our computational reach.

\end{document}
